# Supplementary material for: Using Metadynamics to Reveal Extractant Conformational Free Energy Landscapes
Source: arXiv:2309.06400 source file (2023-12-13)
Supplement: Supplementary file 1 [file SI.pdf]

Support Information: Using Metadynamics to Reveal Extractant Conformational Free Energy Landscapes

Xiaoyu Wang, Michael J. Servis

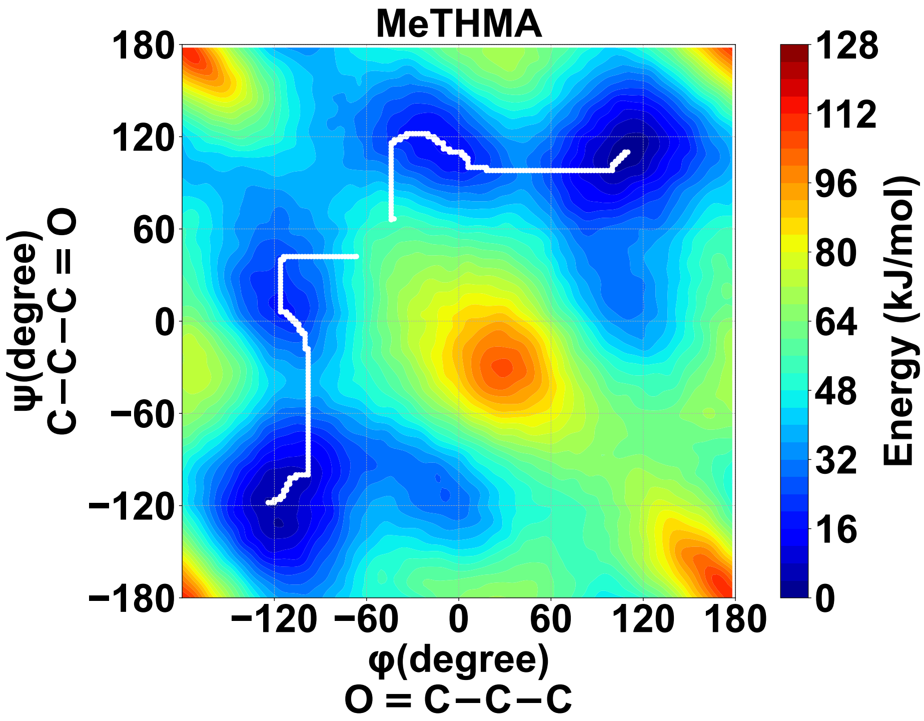


Figure 1S. Bound-to-unbound MFEPs identified on the free energy landscape for MeTHMA.

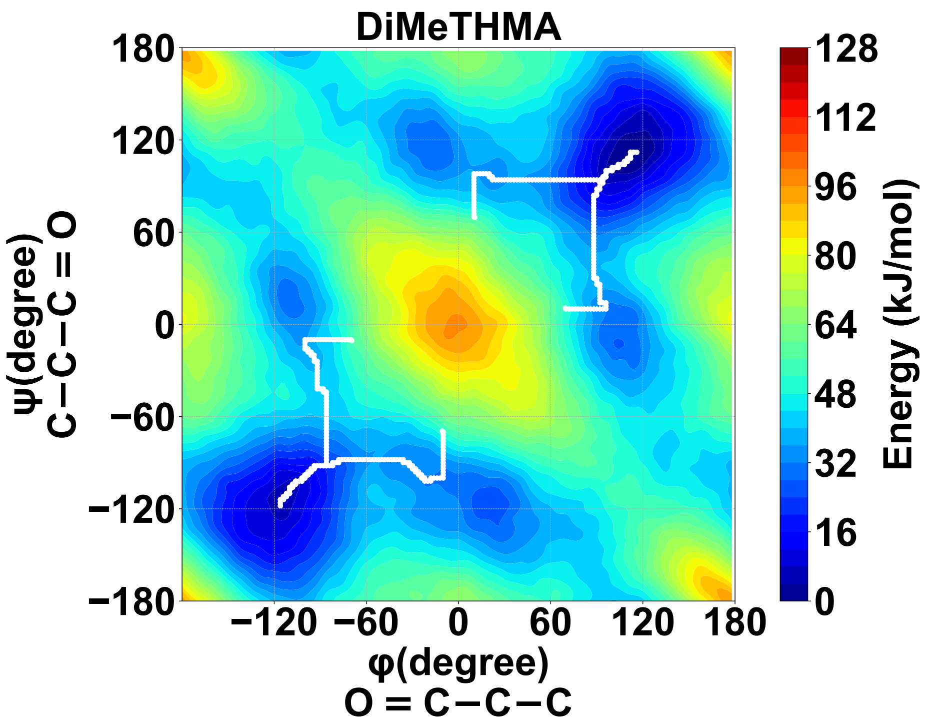


Figure 2S. Bound-to-unbound MFEPs identified on the free energy landscape for DiMeTHMA.

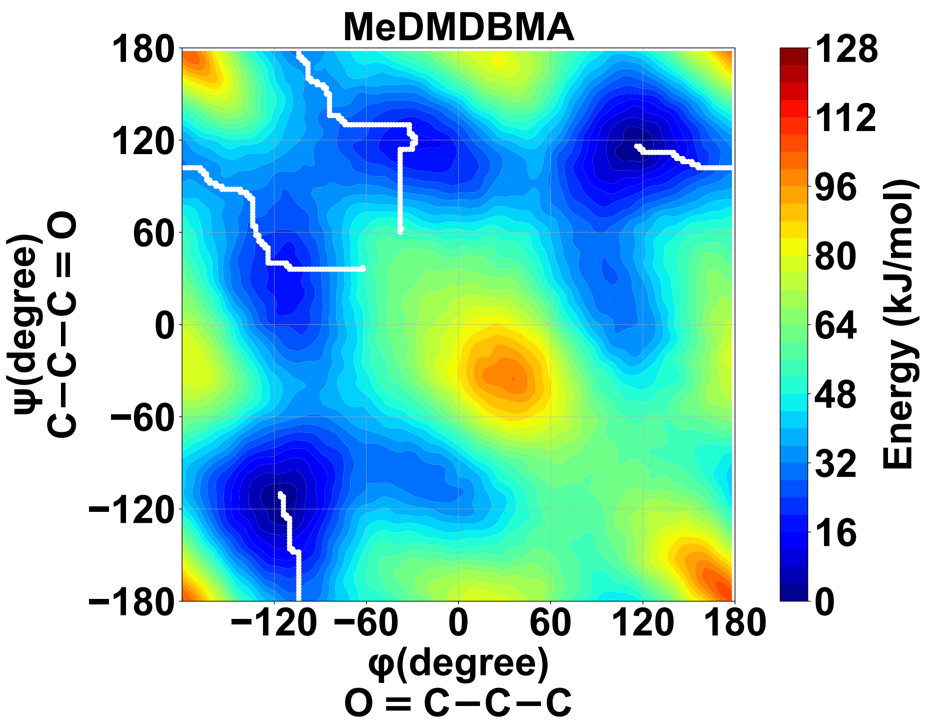


Figure 3S. Bound-to-unbound MFEPs identified on the free energy landscape for MeDMDBMA.

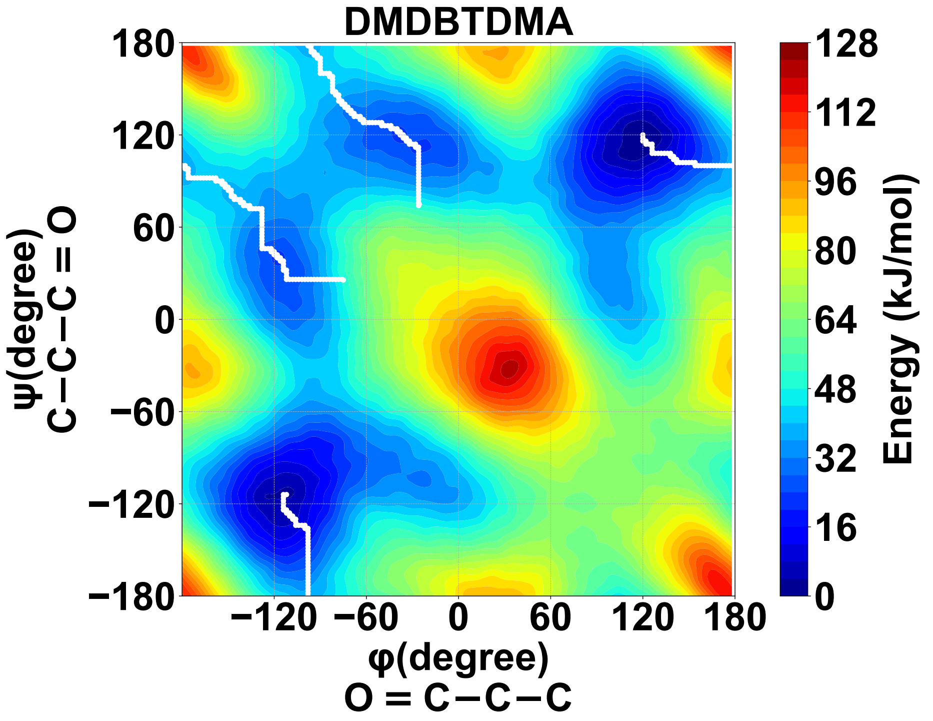


Figure 4S. Bound-to-unbound MFEPs identified on the free energy landscape for DMDBTDMA.

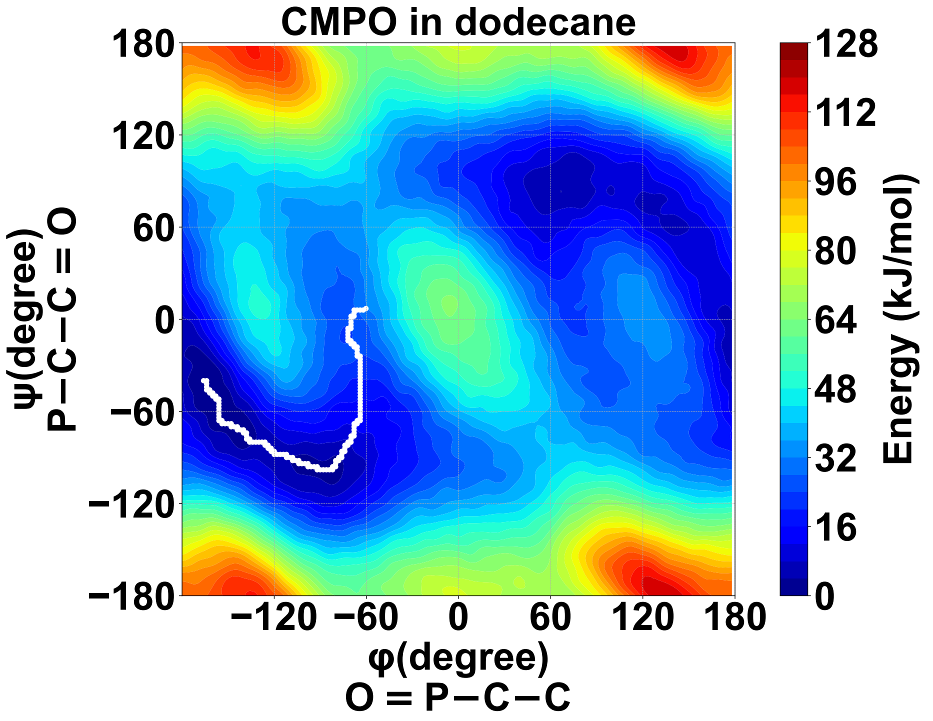


Figure 5S. Bound-to-unbound MFEPs identified on the free energy landscape for CMPO in dodecane.

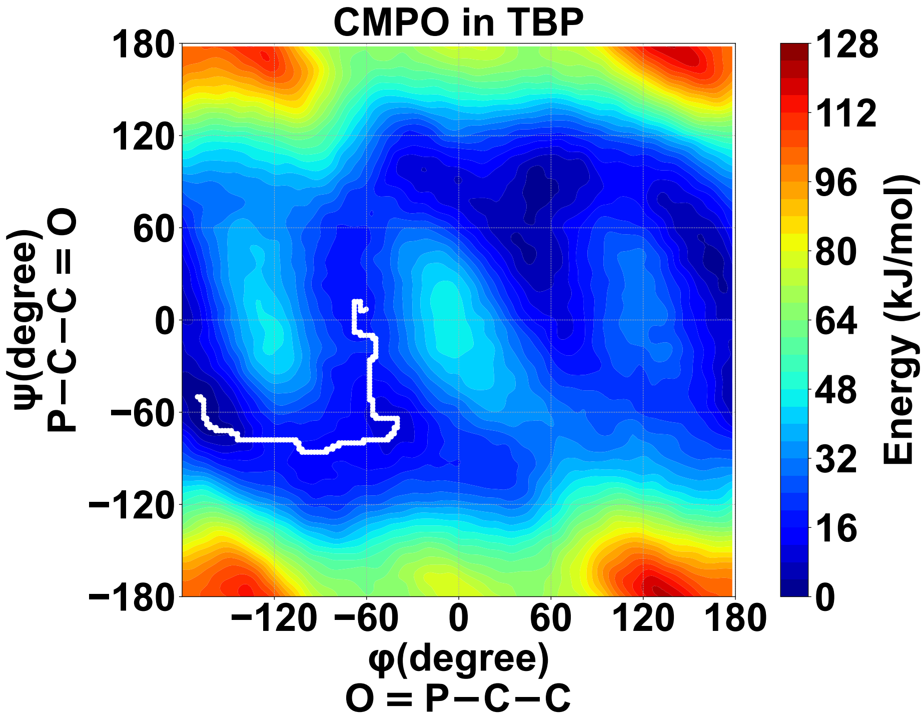

Figure 6S. Bound-to-unbound MFEPs identified on the free energy landscape for CMPO in TBP.
